# Supplementary material for: Adaptive Exploit Generation against Security Devices and Security APIs
Source: arXiv:2410.01568 source file (2024-10-02)
Supplement: Supplementary file 1 [file appendix.tex]

%!TEX root = ../thesis.tex
